# Supplementary material for: Residual Multi-Task Learner for Applied Ranking
Source: arXiv:2411.09705 source file (2024-10-30)
Supplement: Supplementary file 1 [file appendix2.tex]

\section{Detailed Experiment Setting} \label{sec:app-b}

\begin{table*}
    \caption{The list of tuned optimal model configurations. "MLP Structure" specifies the output dimensions of each layer of the employed MLP. "Dropout" indicates the dropout rate applied on MLP hidden layer outputs. "Emb size" denotes the embedding size of each feature. "Pos Sample Weights" details the positive sample weight for each task in multi-task learning, where the negative sample weight is fixed as 1. For KuaiRand-Pure-S1 (Multi-Task), the "Pos Sample Weights" is ordered as [is\_valid\_view, is\_like, is\_follow, is\_comment, is\_forward]. For other datasets, it is ordered according to the task progressiveness.} % Shopee-2 and Shopee-3 are listed in sequence.
    \resizebox{1.0\textwidth}{!}{
    \begin{tabular}{cccccccc}
    \hline
    \hline
    Dataset (Task) & Method & MLP Structure & Dropout & Learning Rate & Emb Size & Batch Size & Pos Sample Weights  \\
    \hline
    \multirow{7}{*}{AliCCP} & NSE & [128, 64, 1] & None & 4e-4 & 32 & 2048 & [1,1000] \\
    & ESMM & [128, 64, 1] & None & 4e-4 & 32 & 2048 & [1,50] \\
    & AITM & [128, 64, 1] & None & 4e-4 & 32 & 2048 & [20,10] \\
    & $\text{ESCM}^2$\text{-IPW} & [128, 64, 1] & None & 4e-4 & 32 & 2048 & [1,50] \\
    & $\text{ESCM}^2$\text{-DR} & [128, 64, 1] & None & 4e-4 & 32 & 2048 & [1,50] \\
    & DCMT & [128, 64, 1] & None & 4e-4 & 32 & 2048 & [1,50] \\
    & ResFlow & [128, 64, 1] & None & 4e-4 & 32 & 2048 & [100,500] \\
    \hline
    \hline
    \multirow{7}{*}{AE} & NSE & [256, 128, 16, 1] & [0.2, 0.2, 0] & 1e-3 & 32 & 1024 & [100,10] \\
    & ESMM & [256, 128, 16, 1] & [0.2, 0.2, 0] & 1e-3 & 32  & 1024 & [50,10] \\
    & AITM & [256, 128, 16, 1] & [0.2, 0.2, 0] & 1e-3 & 32 & 1024 & [100,10] \\
    & $\text{ESCM}^2$\text{-IPW} & [256, 128, 16, 1] & [0.2, 0.2, 0] & 1e-3 & 32 & 1024 & [1,30] \\
    & $\text{ESCM}^2$\text{-DR} & [256, 128, 16, 1] & [0.2, 0.2, 0] & 1e-3 & 32 & 1024 & [1,30] \\
    & DCMT & [256, 128, 16, 1] & [0.2, 0.2, 0] & 1e-3 & 32 & 1024 & [10,50] \\
    & ResFlow & [256, 128, 16, 1] & [0.2, 0.2, 0] & 1e-3 & 32 & 1024 & [1,500] \\
    \hline
    \multirow{7}{*}{Shopee} & NSE & [256, 128, 16] & None & 4e-4  & 16 & 512 & [1,1]; $ $ [1,1,1]\\
    & ESMM & [256, 128, 16] & None & 4e-4 & 16 & 512 & [1,1]; $ $ [1,1,1]\\
    & AITM & [256, 128, 16] & None & 4e-4 & 16 & 512 & [1,1]; $ $ [1,1,1] \\
    & $\text{ESCM}^2$\text{-IPW} & [256, 128, 16] & None &  4e-4 & 16 & 512 & [1,1]; $ $ [1,1,1] \\
    & $\text{ESCM}^2$\text{-DR} & [256, 128, 16]  & None & 4e-4 & 16 & 512 & [1,1]; $ $ [1,1,1] \\
    & DCMT & [256, 128, 16]  & None & 4e-4 & 16 & 512 & [1,1]; $ $ [1,1,1] \\
    & ResFlow & [256, 128, 16] & None  & 4e-4 & 16 & 512 & [1,1]; $ $ [1,1,1] \\
    \hline
    \multirow{3}{*}{MovieLens-1M} & Traditional & [192, 128, 1] & None & 1e-3 & 8 & 512 & NA\\
    & Progressive+NSE & [128, 64, 1] & None & 1e-3 & 8 & 512 & [1,1,1,1,1] \\
    & Progressive+ResFlow & [128, 64, 1] & None & 1e-3 & 8 & 512 & [1,1,1,1,1]  \\
    \hline
    \multirow{3}{8em}{\centering KuaiRand-Pure-S1 (Regression)} & Traditional & [64, 64, 1] & None & 1e-3 & 8 & 512 & NA \\
    & Progressive+NSE & [128, 64, 1] & None & 1e-3 & 8 & 512 & [1,1,1,1,1,1,1,1,1] \\
    & Progressive+ResFlow & [128, 64, 1] & None & 1e-3 & 8 & 512 & [1,1,1,1,1,1,1,1,1]  \\
    \hline
    \multirow{7}{8em}{\centering KuaiRand-Pure-S1 (Multi-Task)} & NSE & [128, 64, 1] & None & 1e-3 & 8 & 512 & [1,1,100,1,40] \\
    & ESMM & [128, 64, 1] & None & 1e-3 & 8 & 512 & [1,20,20,20,20] \\
    & AITM & [128, 64, 1] & None & 1e-3 & 8 & 512 & [1,40,40,40,40]  \\
    & ESCM$^2$-IPW & [128, 64, 1] & None & 1e-3 & 8 & 512 & [1,20,20,20,20] \\
    & ESCM$^2$-DR  & [128, 64, 1] & None & 1e-3 & 8 & 512 & [1,20,20,20,20] \\
    & DCMT & [128, 64, 1] & None & 1e-3 & 8 & 512 & [1,20,20,20,20] \\
    & ResFlow & [128, 64, 1] & None & 1e-3 & 8 & 512 & [1,20,20,20,20]\\
    \hline
    \hline
    \end{tabular}
    }
    \label{tab:reproduce-config}
\end{table*}

We process the AliCCP and AE datasets mainly following prior works~\cite{xi2021modeling,zhu2023dcmt}. For the AliCCP dataset, we parse and use part of the features, including features with ID: 205, 206, 207, 216, 508, 509, 702, 101, 121, 122, 124, 125, 126, 127, 128, 129, 210, and 853. For multi-value categorical features 210 and 853, we use sum pooling to merge the feature embedding before inputting them to MLP. A difference is that we do not filter low-frequency features as they did~\cite{xi2021modeling}. Feature 301 contains the scenario information of this dataset, according to which we split the dataset into multiple subsets. Notably, scenario S2 has no conversion label. For the AE dataset, we parse and use all 62 features. For the four multi-value numeric features, mu1, mu2, mu3, and mu4, we treat them as learned embeddings and feed them directly to the MLP. The dataset is divided into five country-wise subsets, officially. 

For KuaiRand-Pure-S1, we parse and use all 92 features. This dataset contains multiple scenarios, while S1 (data field "tab"=1) takes up about 90\% of the data, making it the largest scenario. We use S1 for our experiments. For the MovieLens-1M dataset, we use all the features. Given the absence of the official split of KuaiRand-Pure-S1 and MovieLens-1M, we order the data samples by timestamp and split the dataset according to the time to simulate real-world scenarios. For MovieLen-1M, we use the foremost 80\% as the train set and the later 20\% as the test set. For KuaiRand-Pure-S1, we use the data in April 2022 as the train set, while using the data in May 2022 as the test set. Similarly, for the Shopee dataset, we use the first 9-day data of Shopee as the train set and the 10th day's data as the test set. 

We discretize all single-value numerical features for all datasets into categorical features, as commonly adopted in industry practice, to stabilize the learning process. 
For all datasets except Shopee, we assign a unique ID for each category in each categorical feature to avoid hashing conflicts in embedding look-up tables. For Shopee, enumerating IDs is impractical, we process the features as introduced in Section \ref{sec:model-robust-over-time}. 

% The dataset statistics are further given in Table \ref{tab:ecommerce-dataset}, \ref{tab:kuairand-dataset}, and \ref{tab:movielen-dataset}.

For the experiments in Section \ref{sec:reg-as-progressive}, the discretizing thresholds for MovieLens-1M are [1, 2, 3, 4, 5], and the discretizing thresholds for KuaiRand-Pure-S1 are [10, 20, 30, 40, 50, 60, 70, 80, 90]. 

For all the models, we use PReLU (negative slope initialized as zero) as the activation unit and Adam ($\beta_1=0.9,\beta_2=0.999$) as the optimizer. We try to use dropout layers between the first two hidden layers in the MLP, but in most cases, this does not improve the performance. We employ a fixed learning rate during the whole training process. We tune all models to get their best performance for each task. For each hyperparameter, we scan the values within a feasible set, e.g., we scan the learning rate in the range [1e-5, 1e-1]. The attained optimal configurations are detailed in Table~\ref{tab:reproduce-config}. 

Notably, for all experiments on the Shopee dataset, we adopt a twin-tower architecture as the backbone network for all tasks and all methods in favor of direct deployment in pre-rank, where we need the twin-tower architecture to speed up model inference. The two towers are implemented as two MLPs that share an identical hidden layer configuration, which is detailed in Table~\ref{tab:reproduce-config}. The two MLPs generate two 16-dimensional vectors, and then the logit of each task is calculated as the inner product of the two vectors. Figure \ref{fig:pre-rank-two-tower}(a) illustrates such twin-tower network architecture, along with how residual connections are incorporated for ResFlow. The 3-target version ResFlow of such twin-tower network architecture is used for online deployment. 

\subsection{Complementary AUC Results}

Complementing the results in the main paper: We provide the AUC results of CTR and ATCR tasks on offline e-commerce datasets in Table~\ref{tab:performance-comparison-ctr-appdx}, \ref{tab:more-baselines2}, and \ref{tab:atcr-result} respectively. ResFlow gets the best mostly. We provide the AUC results for all five tasks in KuaiRand-Pure-S1 multi-task in Table~\ref{tab:Kuairand-multitask-full}. ResFlow gets the best in all tasks. 

\subsection{Probing the ResFlow Residual Learning} 

We offer an alternative visualization of Figure~\ref{fig:case study} by rearranging the feature dimensions according to the average values. The results are shown in Figure~\ref{fig:case-study-2}. We can see that ResFlow has learned a more complex feature utilization spectrum compared to NSE.  

\begin{figure*}
  \centering
  \includegraphics[width=\linewidth]{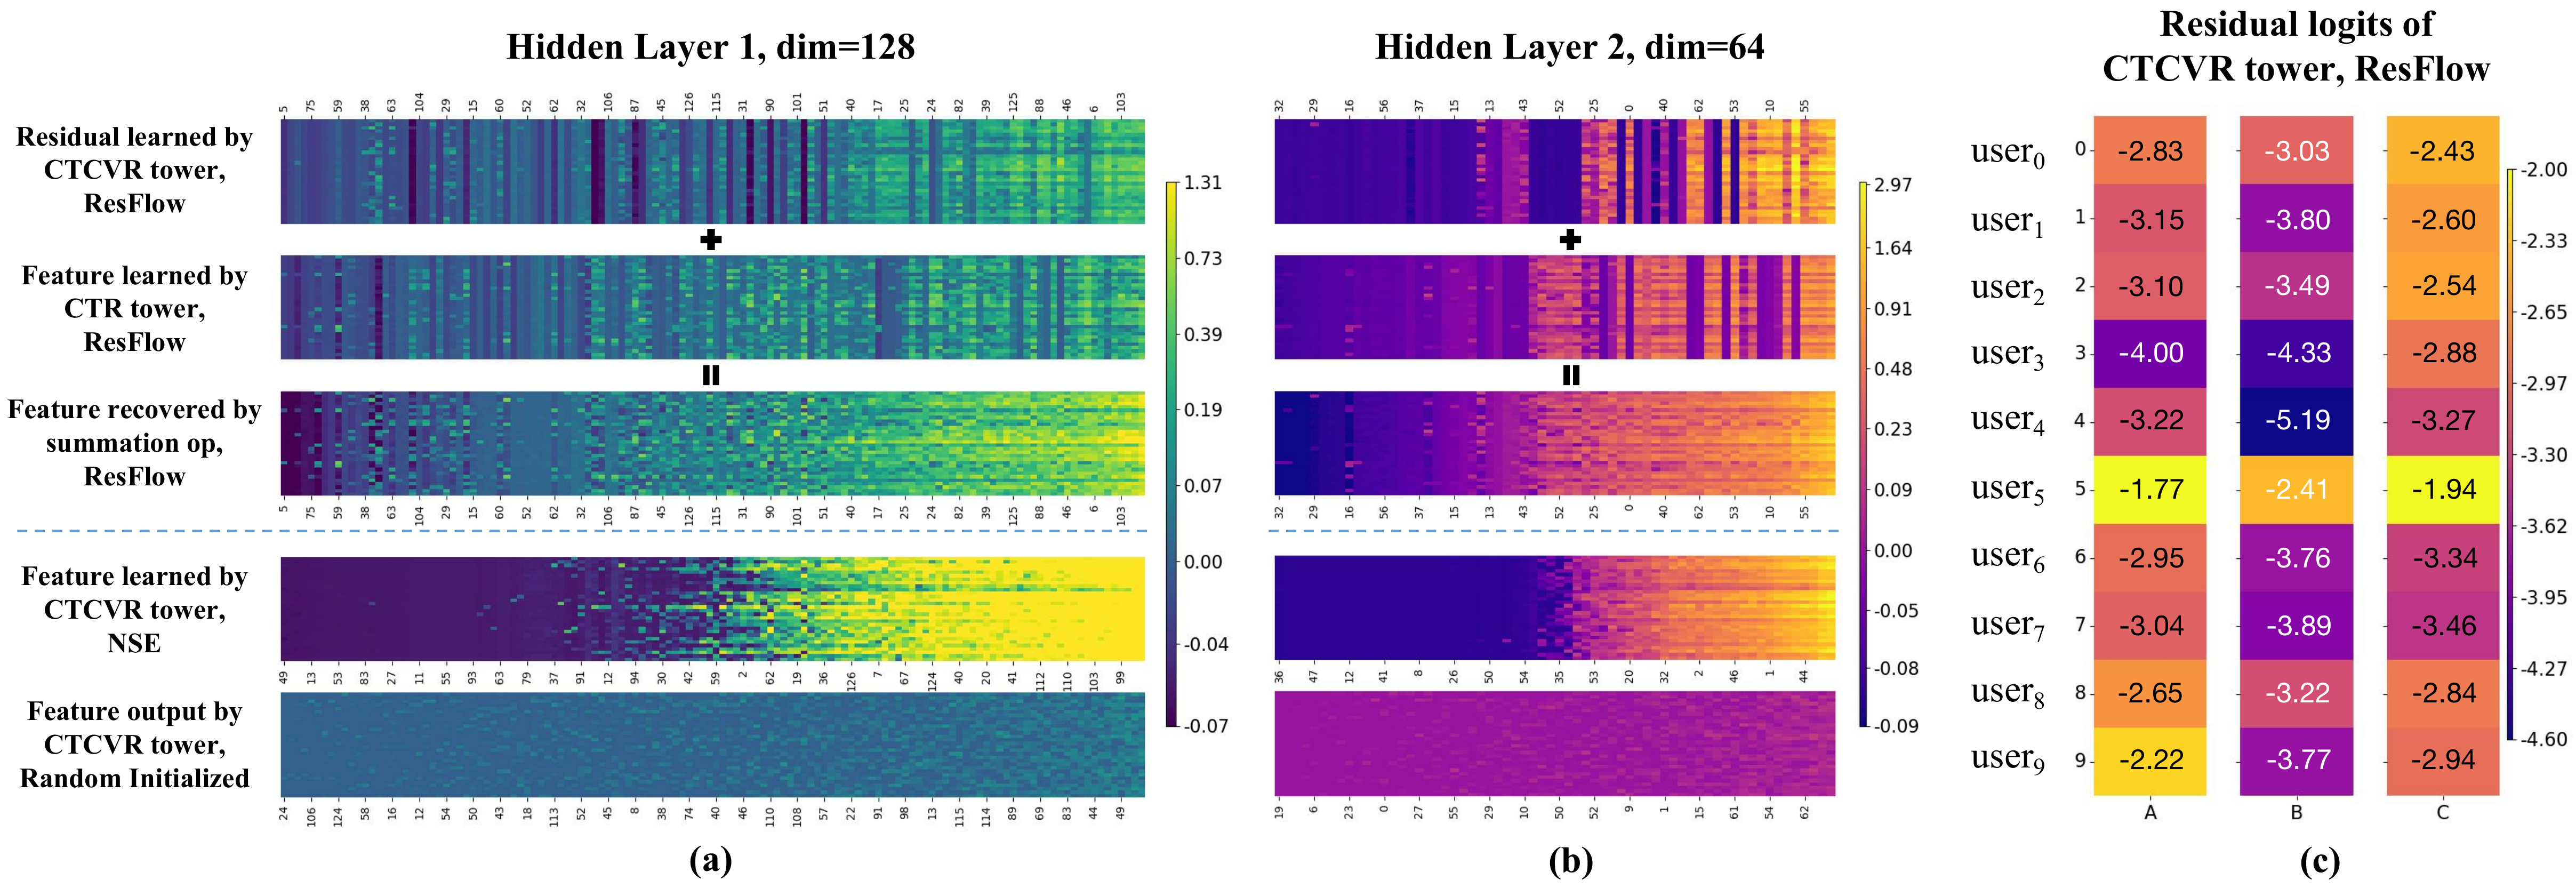}
  \caption{Case study on AliCCP dataset, an alternative visualization of Figure \ref{fig:case study} by sorting the feature dimension according to the average activation values.}
  \label{fig:case-study-2}
\end{figure*}

\section{More on Online Deployment} \label{sec:app_online}

\subsection{Explanation of Additional Offline Metrics}

\subsubsection{NDCG}

The normalized discounted cumulative gain (NDCG) is used to compare the ranked list with an ideally ranked list w.r.t. a certain item scoring function. Here, again, the list to be measured is ranked according to the fused score, while the ideal list is ranked directly according to the item scoring function. The item scoring function in our case is defined by: score(ordered item)=1, score(add-to-cart item)=0.25, score(clicked item)=0.1, and score(no-action item)=0. Then the NDCG is calculated as follows: 
\begin{equation}
    DCG=\sum_{i=1}^n\frac{2^{score(\text{i-th item in the ranking list})}-1}{\log_2(i+1)}, 
\end{equation} 
\begin{equation}
    IDCG=\sum_{j=1}^n\frac{2^{score(\text{j-th item in the ideal ranking list})}-1}{\log_2(j+1)},
\end{equation}
\begin{equation}
    NDCG=\frac{DCG}{IDCG},
\end{equation}
where $n$ is the length of the list. It measures how the ranked list positions relevant items at the top of the list. 

% IDCG and DCG use the same formula for calculation yet with different order. DCG is calculated based on the list ranked with the predicted score, while IDCG is calculated based on the one arranged in the optimal order. 

\subsubsection{List AUC}

Traditionally, AUC is calculated within the task prediction and its corresponding target label, e.g., CTCVR AUC is calculated based on CTCVR task prediction and the "order" labels. It can be defined as the area under the ROC curve, while also can be equivalently defined as the probability that a random positive example is ranked before a random negative example. 
In the deployment of multi-task models, we rank items based on the fused score. We introduce List AUC for our ranking system, using the later definition on the ranked list. List AUC provides a measure of the quality of the ranked list by calculating the probability that a random item with "order" label is ranked before a random item without "order" label. 
List AUC can be calculated with any label. We use the order label because we mainly tune the formula to favor more order placement, i.e., OPU. 

\subsubsection{BCR@K}

The bad case rate at the top K (BCR@K) is a metric by an independent team designed to assess the matchiness of responses (i.e., the final ranked list) to user queries. They conduct this evaluation by comparing the responses provided by the treatment group against a predetermined baseline, i.e., the control group. This process involves sampling 400 queries based on their frequency of occurrence. For each sampled query, the team reviews the top K items of the responded list and tallies the instances of bad cases. One item is considered a bad case if it does not well match the user query. For example: 1) wrong merchandise category, e.g., user searches "iPhone", yet the item is an iPhone case; 2) wrong brand, e.g., user searches "Nike shoes", yet the item is an Adidas shoe; 3) wrong color, e.g., user searches "gray shirts", yet the item is a green shirt; 4) wrong audience, e.g., user searches "shoes women", yet the item is shoes for baby girl, etc. The team then calculates the proportion of bad cases w.r.t. all reviewed cases to get BCR@K, and determines the relative difference using the formula: 
\begin{equation}
\scalemath{0.95}{
    Relative~Difference = \frac{Treatment~Group~BCR@K}{Control~Group~BCR@K} - 1.
}
\end{equation}

\subsection{Non-Smoothed Results of Figure~\ref{fig:online-experiment}} 

In real-world scenarios, the online A/B test results usually fluctuate a lot. We show the non-smoothed version of Figure~\ref{fig:online-experiment} in Figure~\ref{fig:online-experiment3}.

\begin{figure*}
  \centering
  \includegraphics[width=\linewidth]{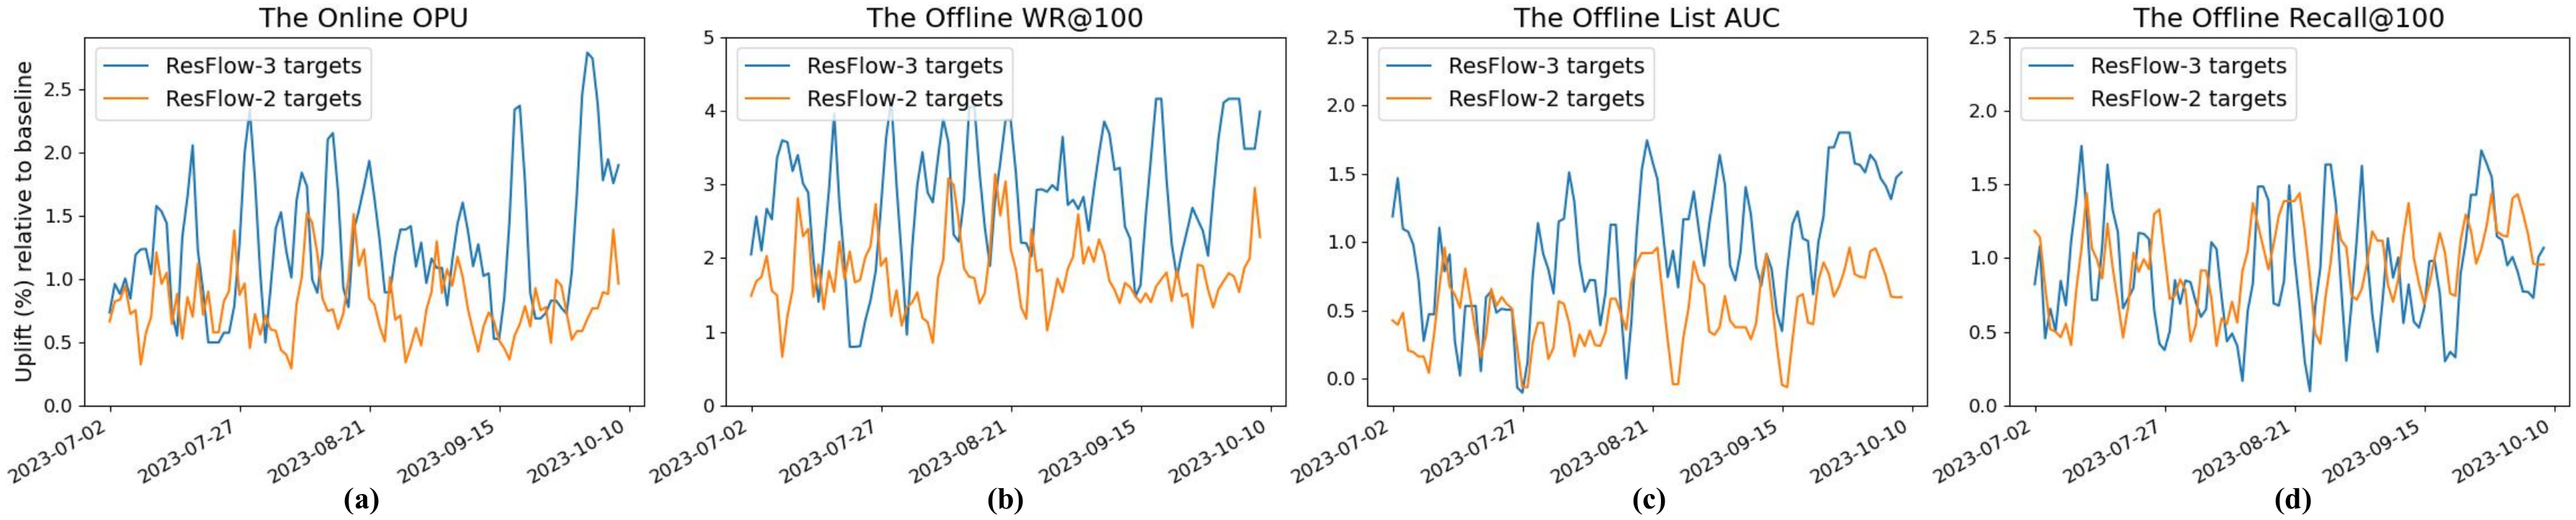}
  \caption{Non-Smoothed Version of Figure~\ref{fig:online-experiment}.}
  \label{fig:online-experiment3}
\end{figure*}

\subsection{Latency Optimization}

The pre-rank stage, tasked with ranking millions of items, has a strict latency upper limit of 150 ms in our scenario. We optimized system latency to maximize model potential. We have identified that embedding lookup is the primary latency contributor, due to a large embedding table (approximately 1 billion embeddings, taking up 99\% of the model parameters). In standard TensorFlow serving, this caused frequent page faults. Our solution involved a dedicated distributed embedding server cluster, each server loading a segment of the embedding table. During inference, categorical feature keys are parallel-retrieved from these servers. For further optimization, techniques like lock-free hash tables, SIMD instructions, and BRPC network protocol enhancements are included. 
Compared to standard TensorFlow serving, our approach supports a ten times larger embedding table within the same latency (20 ms), which led to a 2\% AUC uplift on test sets, due to reduced hashing conflicts. 

\subsection{Training Data Curation}

Effective training data curation is crucial for the pre-rank stage, especially considering that approximately 99\% of items input to the pre-rank are not viewed. Training solely on viewed data leads to a significant mismatch between the online-serving input distribution and the training distribution. To align these distributions, we curated samples from various system modules: 
% and manage the sample size for training with limited resources 

\begin{itemize}[leftmargin=*]
\item \textbf{Viewed Samples (D1)}: From the serving log, viewed samples, containing user feedback. 
\item \textbf{Unviewed Rank Candidates (D2)}: From the rank server log, items that were not viewed. Used as negative samples. 
\item \textbf{Unviewed Pre-Rank Candidates (D3)}: From the match engine log, items that did not pass the match engine's truncation and thus didn't reach the rank stage. Used as negative samples. 
\item \textbf{Random Samples (D4)}: Selected through random sampling from the entire item set. Used as negative samples. 
\end{itemize}

% \textbf{Asymmetric Testing:} The traditional test setting, which involves assessing models on untrained future train sets, is not apt for our scenario since the pre-rank training set may not accurately represent the actual online distribution. Additionally, due to the high cost, dumping the full pre-rank traffic log is not feasible. Therefore, to create a more accurate testing environment, we selectively sampled and analyzed a portion of the pre-rank traffic logs, namely the \textbf{AsymSet}. 

As shown in Table \ref{tab:data-curation}, omitting unviewed pre-rank (D3) and unviewed rank (D2) candidates leads to a significant drop in offline CTCVR AUC and WR@100. This indicates the importance of these negative items in training the model. Whereas removing random samples does not substantially impact CTCVR AUC or WR@100 but reduces the rate of bad cases. This suggests that some recall strategies, such as personalized recall and similar-keyword-based item recall, may introduce items misaligned with the current keyword intention. Random negative samples help the model differentiate such unintended items, thus improving the user experience. 

\begin{table}
    \caption{Ablation Study on Train Data for Pre-Rank Module.} 
    % We mainly observe the change in main offline metrics WR@100 (order-based) and CTCVR AUC, and user experience metrics bad-case rate @20 of rank output (BCR@20). 
    % The BCR@20 counts the proportion of irrelevant items within the top 20 rank outputs with 400 randomly sampled keywords.} 
    \begin{tabular}{cccc}
    \hline
    \hline
    Dataset & WR@100 & CTCVR AUC & BCR@20 \\
    \hline
    D1 & 0.587 & 0.812 & 0.089 \\
    D1 + D2 & 0.663 & 0.916 &  0.090 \\
    D1 + D2 + D3 & 0.711 & 0.951 & 0.088  \\
    D1 + D2 + D3 + D4 & 0.714 & 0.953 & 0.061 \\
    \hline
    \hline
    \end{tabular}
    \label{tab:data-curation}
\end{table}

\subsection{Model Robustness Over Time}
\label{sec:model-robust-over-time}

Maintaining model robustness over time in response to evolving user preferences is challenging due to factors like data distribution shifts, merchandise life-cycle impacts, and training overfit. We developed several strategies to address these issues:
\begin{itemize}[leftmargin=*]
    \item \textbf{Discretization of Numeric Features}: To counter the impact of significant shifts in numeric feature values over time, we bucketize these features, virtually transforming them into categorical features. This helps alleviate data distribution shift issues. 
    
    \item \textbf{Embedding Filter and Eviction}: With millions of items going on and off the shelf every day, unrestrained growth in the model size is unsustainable, potentially increasing by 10 GB weekly. Moreover, new items often have under-fit embeddings due to limited user interactions, affecting model stability. To counter this, we create new embedding table entries only for IDs appearing more than $m$ times in training data and evict IDs absent from the training data for the past $n$ days. IDs without an entry are mapped to a default embedding for each feature. We tune $m$ and $n$ to reduce the negative impact on the model test metric and reduce the performance variance of daily training. 
    
    \item \textbf{One Epoch Training}: As found in \cite{zhang2022towards}, our model tends to overfit with more than one epoch of daily incremental training. Therefore, we limit training to one epoch per day's data. 
\end{itemize}

\noindent These led to a reduction in the standard deviation of offline WR@100 and List AUC in "next-day testing" by 0.01 and 0.004, respectively. In a two-week online A/B test, the standard deviation of online OPU decreased by 0.002, while the average OPU uplift is slightly better (+0.2\%) than the baseline without these strategies. 

% \begin{table*}
% \caption{Ablation results of ResFlow in terms of CTCVR AUC.}
% \begin{tabular}{ccccc}
% \hline
% \hline
% Model                       &        AliCCP       &        AE-RU        &       Shopee-2      \\
% \hline
% NSE                         & 0.6238 $\pm$ 0.0018 & 0.8692 $\pm$ 0.0032 & 0.8648 $\pm$ 0.0012 \\
% NSE + Feature Residual (FR) & 0.6482 $\pm$ 0.0010 & 0.8969 $\pm$ 0.0013 & 0.8909 $\pm$ 0.0011 \\
% NSE + FR(H1-only)           & 0.6296 $\pm$ 0.0021 & 0.8797 $\pm$ 0.0021 & 0.8682 $\pm$ 0.0016 \\
% NSE + FR(H2-only)           & 0.6417 $\pm$ 0.0015 & 0.8983 $\pm$ 0.0019 & 0.8873 $\pm$ 0.0013 \\
% NSE + Logit Residual (LR)   & 0.6511 $\pm$ 0.0013 & 0.9065 $\pm$ 0.0017 & 0.8963 $\pm$ 0.0014 \\
% ResFlow(NSE + FR + LR)      & 0.6642 $\pm$ 0.0016 & 0.9134 $\pm$ 0.0015 & 0.9024 $\pm$ 0.0010 \\
% ESMM                        & 0.6412 $\pm$ 0.0031 & 0.8778 $\pm$ 0.0022 & 0.8817 $\pm$ 0.0010 \\
% ESMM + FR                   & 0.6503 $\pm$ 0.0028 & 0.8991 $\pm$ 0.0037 & 0.8912 $\pm$ 0.0017 \\
% ESMM + FR + LR              & 0.6487 $\pm$ 0.0043 & 0.8963 $\pm$ 0.0061 & 0.8881 $\pm$ 0.0011 \\
% \hline
% \hline
% \end{tabular}
% \label{tab:more-ablation}
% \end{table*}

\begin{table*}
    \caption{The AUC results of the CTR estimation task on offline e-commerce datasets.} 
    \begin{tabularx}{1\textwidth}{
        >{\centering\arraybackslash}m{3.8em}
        >{\centering\arraybackslash}m{6.2em}
        >{\centering\arraybackslash}m{6.2em}
        >{\centering\arraybackslash}m{6.2em}
        >{\centering\arraybackslash}m{6.2em}
        >{\centering\arraybackslash}m{6.2em}
        >{\centering\arraybackslash}m{6.2em}
        >{\centering\arraybackslash}m{6.2em}
    }
    \hline
    \hline
    Dataset & NSE & AITM & ESMM & ESCM$^2$-IPW & ESCM$^2$-DR & DCMT & ResFlow (ours) \\
    \hline
    S0 & \underline{$0.5957\pm0.0023$} & $0.5934\pm0.0013$ & $0.5921\pm0.0017$ & $0.5835\pm0.0017$ & $0.5847\pm0.0029$ & $0.5909\pm0.0031$ & $\mathbf{0.5971\pm0.0011}$ \\    
    S1 & $\mathbf{0.6151\pm0.0039}$ & $0.6071\pm0.0041$ & $0.6075\pm0.0016$ & $0.5655\pm0.0032$ & $0.5672\pm0.0028$ & $0.6008\pm0.0027$ & \underline{$0.6128\pm0.0031$} \\    
    S0\&S1 & $0.5968\pm0.0011$ & $0.5936\pm0.0009$ & $0.5915\pm0.0029$ & $0.5724\pm0.0013$ & $0.5752\pm0.0017$ & $\underline{0.5982\pm0.0022}$ & $\mathbf{0.5993\pm0.0006}$ \\    
    AliCCP & $0.6029\pm0.0037$ & $\underline{0.6039\pm0.0011}$ & $0.5959\pm0.0012$ & $0.5810\pm0.0015$ & $0.5835\pm0.0025$ & $0.5928\pm0.0036$ & $\mathbf{0.6045\pm 0.0013}$\\    
    \hline
    AE-ES & $0.7270\pm0.0042$ & $0.7281\pm0.0047$ & $0.7240\pm0.0025$ & $0.7224\pm0.0027$ & $0.7274\pm0.0011$ & $\underline{0.7296\pm0.0034}$ & $\mathbf{0.7299\pm0.0029}$ \\    
    AE-FR & $0.7194\pm0.0043$ & $\mathbf{0.7237\pm0.0022}$ & $0.7184\pm0.0027$ & $0.7210\pm0.0036$ & $0.72044\pm0.0014$ & $0.7216\pm0.0027$ & \underline{$0.7223\pm0.0023$} \\    
    AE-NL & $0.7100\pm0.0021$ & $0.7119\pm0.0010$ & $0.7098\pm0.0021$ & $0.7096\pm0.0014$ & $0.7076\pm0.0022$ & $\underline{0.7138\pm0.0021}$ & $\mathbf{0.7139\pm0.0016}$ \\    
    AE-US & $0.7036\pm0.0023$ & $0.7009\pm0.0035$ & $0.7001\pm0.0027$ & $0.6994\pm0.0013$ & $0.7009\pm0.0037$ & $\underline{0.7040\pm0.0020}$ & $\mathbf{0.7055\pm0.0026}$ \\    
    AE-RU & $0.7331\pm0.0019$ & $0.7330\pm0.0048$ & $0.7342\pm0.0011$ & $0.7339\pm0.0008$ & $\mathbf{0.7369\pm0.0017}$ & $0.7318\pm0.0016$ & \underline{$0.7351\pm0.0022$} \\
    \hline
    Shopee-2 & $\underline{0.8628\pm0.0009}$ & $0.8452\pm0.0011$ & $0.8493\pm0.0017$ & $0.8283\pm0.0063$ & $0.8567\pm0.0013$ & $0.8597\pm0.0039$ & $\mathbf{0.8667\pm0.0014}$ \\    
    Shopee-3 & $0.8551\pm0.0027$ & $0.8553\pm0.0016$  & $\underline{0.8650\pm0.0032}$ & / & / & / & $\mathbf{0.8692\pm0.0022}$ \\
    \hline
    \hline
    \end{tabularx}
    \label{tab:performance-comparison-ctr-appdx}
\end{table*}

\begin{table*}
    \caption{More AUC results of the CTR estimation task on offline e-commercial datasets.}
    \begin{tabular}{ccccc}
    \hline
    \hline
    Datasets &Single Task& MOE & MMOE & PLE \\
     S0    &0.5911 $\pm$ 0.0024& 0.5962 $\pm$ 0.0010 & 0.5955 $\pm$ 0.0021 & 0.5956 $\pm$ 0.0011 \\
     S1    &0.6119 $\pm$ 0.0019& 0.6116 $\pm$ 0.0008 & 0.6124 $\pm$ 0.0036 & 0.6120 $\pm$ 0.0017 \\
     S0\&S1 &0.5966 $\pm$ 0.0015& 0.5988 $\pm$ 0.0021 & 0.5979 $\pm$ 0.0019 & 0.5981 $\pm$ 0.0023 \\
     AliCCP&0.5998 $\pm$ 0.0021& 0.6038 $\pm$ 0.0024 & 0.6021 $\pm$ 0.0020 & 0.6033 $\pm$ 0.0014 \\
     \hline
     AE-ES &0.7285 $\pm$ 0.0017& 0.7283 $\pm$ 0.0013 & 0.7289 $\pm$ 0.0027 & 0.7294 $\pm$ 0.0023 \\
     AE-FR &0.7231 $\pm$ 0.0020& 0.7239 $\pm$ 0.0028 & 0.7225 $\pm$ 0.0031 & 0.7208 $\pm$ 0.0022 \\
     AE-NL &0.7121 $\pm$ 0.0035& 0.7091 $\pm$ 0.0019 & 0.7118 $\pm$ 0.0022 & 0.7136 $\pm$ 0.0031 \\
     AE-US &0.7029 $\pm$ 0.0029& 0.7012 $\pm$ 0.0012 & 0.7011 $\pm$ 0.0021 & 0.7033 $\pm$ 0.0010 \\
     AE-RU &0.7343 $\pm$ 0.0012& 0.7323 $\pm$ 0.0025 & 0.7334 $\pm$ 0.0009 & 0.7331 $\pm$ 0.0034 \\
     \hline
     Shopee-2&0.8522 $\pm$ 0.0008& 0.8479 $\pm$ 0.0006 & 0.8482 $\pm$ 0.0016 & 0.8504 $\pm$ 0.0012 \\
     Shopee-3&0.8522 $\pm$ 0.0008& 0.8567 $\pm$ 0.0021 & 0.8569 $\pm$ 0.0011 & 0.8592 $\pm$ 0.0008 \\
     \hline
    \hline
    \end{tabular}
    \label{tab:more-baselines2}
\end{table*}

\begin{table*}
    \caption{Multi-task Performance on KuaiRand-Pure-S1 in terms of AUC.}
    \begin{tabular}{cccccc}
    \hline
    \hline
    Target & is\_valid\_view & is\_like & is\_follow & is\_comment & is\_forward \\
    \hline
    Single Task  & 0.6639 $\pm$ 0.0012 & 0.8693 $\pm$ 0.0038 & 0.7765 $\pm$ 0.0052 & 0.7594 $\pm$ 0.0031 & 0.7262 $\pm$ 0.0047 \\
    NSE& $0.6617\pm0.0008$ & $0.8729\pm0.0016$ & $0.8210\pm0.0045$ & $0.7790\pm0.0029$ & $0.7501\pm0.0106$\\
    MOE & 0.6634 $\pm$ 0.0026 & 0.8713 $\pm$ 0.0017 & 0.8019 $\pm$ 0.0046 & 0.7803 $\pm$ 0.0021 & 0.7533 $\pm$ 0.0053 \\
    MMOE & 0.6622 $\pm$ 0.0013 & 0.8689 $\pm$ 0.0022 & 0.8111 $\pm$ 0.0028 & 0.7797 $\pm$ 0.0031 & 0.7595 $\pm$ 0.0039 \\
    PLE & 0.6629 $\pm$ 0.0031 & 0.8709 $\pm$ 0.0019 & 0.8208 $\pm$ 0.0030 & 0.7781 $\pm$ 0.0044 & 0.7601 $\pm$ 0.0043 \\
    
    ESMM& $0.6629\pm0.0019$ & $0.8744\pm0.0024$ & \underline{$0.8221\pm0.0072$} & $0.7818\pm0.0040$ & $0.7572\pm0.0071$\\
    
    AITM& $0.6633\pm0.0015$ & $0.8741\pm0.0017$ & $0.7845\pm0.0142$ & $0.7821\pm0.0047$ & \underline{$0.7639\pm0.0118$}\\
    
    $\text{ESCM}^2$\text{-IPW}& $0.6623\pm0.0011$ & \underline{$0.8758\pm0.0011$} & $0.8170\pm0.0101$ & $0.7729\pm0.0040$ & $0.7541\pm0.0079$\\
    
    $\text{ESCM}^2$\text{-DR}& $0.6616\pm0.0016$ & $0.8753\pm0.0013$ & $0.8206\pm0.0098$ & $0.7824\pm 0.0027$ & $0.7538\pm0.0083$\\
    
    DCMT & $\underline{0.6636\pm0.0021}$ & $0.8743\pm0.0019$ & $0.8194\pm0.0069$ & \underline{$0.7830\pm0.0026$} & $0.7623\pm0.0083$\\
    
    ResFlow & $\mathbf{0.6642\pm0.0014}$ & $\mathbf{0.8759\pm0.0009}$ & $\mathbf{0.8257\pm0.0022}$ & $\mathbf{0.7886\pm0.0028}$ & $\mathbf{0.7762\pm0.0059}$\\
    \hline
    \hline
    \end{tabular}
    \label{tab:Kuairand-multitask-full}
\end{table*}

\begin{table*}
    \caption{ATCR AUC results on Shopee-3.} %We exclude ESCM$^2$ and DCMT due to their failure in the training process as mentioned in the main text. AUC-avg denotes the average of the ATCR AUC, while AUC-std denotes its standard derivation.
    \begin{tabular}{ccccc}
    \hline
    \hline
     Method & NSE & ATIM & ESMM & ResFlow \\ 
    \hline
     AUC & $0.8679 \pm 0.0013$ & $0.8715 \pm 0.0021$ & $0.8753 \pm 0.0017$ & $0.8864 \pm 0.0015$ \\ 
     % AUC-std & 0.0013 & 0.0021 & 0.0017 & 0.0015 \\ 
    \hline
    \hline
    \end{tabular}
    \label{tab:atcr-result}
\end{table*}
