# Supplementary material for: Residual Multi-Task Learner for Applied Ranking
Source: arXiv:2411.09705 source file (2024-10-30)
Supplement: Supplementary file 2 [file appendix_bak.tex]

\section{Appendices}

Teaser figure: Illustrating possibly more complex scenarios in the Appendix.

  - conceptual architecture of ResFlow for other topology
    1) tow-tower, i.e., pre-rank
    2) formed by resnet blocks
    4) formed by inception blocks
    
Appendix A: Detailed experiment setting
   
  - Due to page limitations, we provide more detailed information about the datasets and implementations in the Appendix. 

Appendix B: More experiment results

  - The results for other tasks, e.g., CTR estimation, are provided in the Appendix, where we can see that ResFlow also gets the best. % approximately.

  - The full table with AUCs of all tasks is provided in the Appendix. 
  
  - Additional experiments. 
        1) forcing negative; 
        2) WR@K variant and its results; 
        3) non-smoothed result of Figure 5; 
        4) results of other task topological structures for sec 4.5; visualizing task topology

Appendix C: More about online deployment

  - explanation of List AUC, NDCG, BCR. 
  
  - dataset curation; latency optimization; robustness over time;




\subsection{Detailed experiment setting}
Due to page limitations, we provide more detailed information about the datasets and implementations in the Appendix.
\label{sec:detailed-exp}
\textbf{Dataset Process.} We process AliCCP and AE datasets following prior works~\cite{xi2021modeling,zhu2023dcmt}. The differences are that we do not filter low-frequency categorical features and we bucketize all numerical features into categorical features as what we do in industry practice. We use the official train-test split for AliCCP and AE. Considering the absence of official split of KuaiRand-Pure-S1 and MovieLens-1M, we order the data samples by timestamp and use 80\% data in the past as train set while 20\% in the future as test set. Similarly, we use the first 9-day data of Shopee as train set while the 10th day as test set. 

\noindent \textbf{Model Configuration.} We sufficiently tune all models to get their best performance for each task. The corresponding configuration are detailed in Table \ref{tab:reproduce-config}.


\begin{table*}[h]
\centering
\caption{Optimal model configurations across all datasets. 'MLP Structure' specifies the output dimensions of each layer, from input to output. 'Dropout' indicates the dropout rate applied between MLP hidden layers. 'Weights' details the 'positive:negative' sample weight for each binary task in multi-task learning. For e-commerce datasets, weight configurations follow the [CTR, CTCVR] sequence. For KuaiRand-MultiTask, weights are ordered as [is\_like, is\_follow, is\_comment, is\_forward].}
\begin{tabular}{cccccccc}
\hline
\hline
Dataset & Method & MLP Structure & Dropout & Learning Rate & Emb Size & Batch Size & Weights  \\
\hline
\multirow{7}{*}{AliCCP} & NSE & [128, 64, 1] & None & 4e-4 & 32 & 2048 & [1:1,1000:1] \\
& ESMM & [128, 64, 1] & None & 4e-4 & 32 & 2048 & [1:1,50:1] \\
& AITM & [128, 64, 1] & None & 4e-4 & 32 & 2048 & [20:1,10:1] \\
& $\text{ESCM}^2$\text{-IPW} & [128, 64, 1] & None & 4e-4 & 32 & 2048 & [1:1,50:1] \\
& $\text{ESCM}^2$\text{-DR} & [128, 64, 1] & None & 4e-4 & 32 & 2048 & [1:1,50:1] \\
& DCMT & [128, 64, 1] & None & 4e-4 & 32 & 2048 & [1:1,50:1] \\
& ResFlow & [128, 64, 1] & None & 4e-4 & 32 & 2048 & [100:1,500:1] \\
\hline
\hline
\multirow{7}{*}{AE} & NSE & [256, 128, 16, 1] & [0.2, 0.2] & 1e-3 & 32 & 1024 & [100:1,10:1] \\
& ESMM & [256, 128, 16, 1] & [0.2, 0.2] & 1e-3 & 32  & 1024 & [50:1,10:1] \\
& AITM & [256, 128, 16, 1] & [0.2, 0.2] & 1e-3 & 32 & 1024 & [100:1,10:1] \\
& $\text{ESCM}^2$\text{-IPW} & [256, 128, 16, 1] & [0.2, 0.2] & 1e-3 & 32 & 1024 & [1:1,30:1] \\
& $\text{ESCM}^2$\text{-DR} & [256, 128, 16, 1] & [0.2, 0.2] & 1e-3 & 32 & 1024 & [1:1,30:1] \\
& DCMT & [256, 128, 16, 1] & [0.2, 0.2] & 1e-3 & 32 & 1024 & [10:1,50:1] \\
& ResFlow & [256, 128, 16, 1] & [0.2, 0.2] & 1e-3 & 32 & 1024 & [1:1,500:1] \\
\hline
\multirow{7}{*}{Shopee} & NSE & [256, 128, 16, 1] & None & 5e-4  & 16 & 512 & [1:1,1:1] \\
& ESMM & [256, 128, 16, 1] & None & 5e-4 & 16 & 512 & [1:1,1:1]\\
& AITM & [256, 128, 16, 1] & None & 5e-4 & 16 & 512 & [1:1,1:1] \\
& $\text{ESCM}^2$\text{-IPW} & [256, 128, 16, 1] & None &  5e-4 & 16 & 512 & [1:1,1:1] \\
& $\text{ESCM}^2$\text{-DR} & [256, 128, 16, 1]  & None & 5e-4 & 16 & 512 & [1:1,1:1] \\
& DCMT & [256, 128, 16, 1]  & None & 5e-4 & 16 & 512 & [1:1,1:1] \\
& ResFlow & [256, 128, 16, 1] & None  & 5e-4 & 16 & 512 & [1:1,1:1] \\
\hline
\multirow{3}{*}{MovieLens-1M} & Traditional & [192, 128, 1] & None & 1e-3 & 8 & 512 & NA\\
& Progressive+NSE & [128, 64, 1] & None & 1e-3 & 8 & 512 & NA \\
& Progressive+ResFlow & [128, 64, 1] & None & 1e-3 & 8 & 512 & NA  \\
\hline
\multirow{3}{*}{KuaiRand-Regression} & Traditional & [64, 64, 1] & None & 1e-3 & 8 & 512 & NA \\
& Progressive+NSE & [128, 64, 1] & None & 1e-3 & 8 & 512 & NA \\
& Progressive+ResFlow & [128, 64, 1] & None & 1e-3 & 8 & 512 & NA  \\
\hline
\multirow{7}{*}{KuaiRand-MultiTask} & NSE & [128, 64, 1] & None & 1e-3 & 8 & 512 & [1:1,100:1,1:1,40:1] \\
& ESMM & [128, 64, 1] & None & 1e-3 & 8 & 512 & [20:1,20:1,20:1,20:1] \\
& AITM & [128, 64, 1] & None & 1e-3 & 8 & 512 & [40:1,40:1,40:1,40:1]  \\
& ESCM$^2$-IPW & [128, 64, 1] & None & 1e-3 & 8 & 512 & [20:1,20:1,20:1,20:1] \\
& ESCM$^2$-DR  & [128, 64, 1] & None & 1e-3 & 8 & 512 & [20:1,20:1,20:1,20:1] \\
& DCMT & [128, 64, 1] & None & 1e-3 & 8 & 512 & [20:1,20:1,20:1,20:1] \\
& ResFlow & [128, 64, 1] & None & 1e-3 & 8 & 512 & [20:1,20:1,20:1,20:1]\\
\hline
\hline
\end{tabular}
\label{tab:reproduce-config}
\end{table*}

% \begin{table*}[h]
% \centering
% \caption{MovieLens-1M Rating Regression Configuration}
% \begin{tabular}{cccc}
% \hline
% \hline
% Configuration & Emb Size & MLP Structure \\
% \hline
% MLP + Integral & 8 & [128, 64, 1] \\
% \hline
% Regression & 8 & [128, 64, 1] \\
% \hline
% Regression-fat & 8 & [256, 128, 1] \\
% \hline
% ResFlow + Integral & 8 & [128, 64, 1] \\
% \hline
% \hline
% \end{tabular}
% \label{tab:reproduce-movielens}
% \end{table*}

% \begin{table*}[h]
% \centering
% \caption{KuaiRand-pure S1 Video Play-Time Regression Configuration}
% \begin{tabular}{cccc}
% \hline
% \hline
% Configuration & Emb Size & MLP Structure & Discretization Interval \\
% \hline
% MLP + Integral & 8 & [128, 64, 1]  & [10, 20, 30, 40, 50, 60, 70, 80, 90]\\
% \hline
% Regression & 8 & [128, 64, 1]  & --\\
% \hline
% Regression-fat & 8 & [384, 192, 1]  & --\\
% \hline
% ResFlow + Integral & 8 & [128, 64, 1]  & [10, 20, 30, 40, 50, 60, 70, 80, 90]\\
% \hline
% \hline
% \end{tabular}
% \label{tab:reproduce-Kuairand-playtime}
% \end{table*}


% \begin{table*}[h]
% \centering
% \caption{KuaiRand-pure S1 Multitask Model Configuration. CXRs are arranged in the order of:[is\_like, is\_follow, is\_comment, is\_forward]}
% \begin{tabular}{cccc}
% \hline
% \hline
% Configuration & Emb Size & Dense Layer & CXR Postive:Negative Weight \\
% \hline
% MLP & 8 & [128, 64, 1] & [1:1,100:1,1:1,40:1]\\
% \hline
% ESMM & 8 & [128, 64, 1] & [20:1,20:1,20:1,20:1]\\
% \hline
% AITM & 8 & [128, 64, 1] &  [40:1,40:1,40:1,40:1]\\
% \hline
% $\text{ESCM}^2$\text{-IPW} & 8 & [128, 64, 1] &  [20:1,20:1,20:1,20:1]\\
% \hline
% $\text{ESCM}^2$\text{-DR} & 8 & [128, 64, 1] &  [20:1,20:1,20:1,20:1]\\
% \hline
% DCMT & 8 & [128, 64, 1] &  [20:1,20:1,20:1,20:1]\\
% \hline
% ResFlow & 8 & [128, 64, 1] &  [20:1,20:1,20:1,20:1]\\
% \hline
% \hline
% \end{tabular}
% \label{tab:reproduce-Kuairand-multitask}
% \end{table*}

\subsection{More experiment results}



\subsection{Case study}
The case study on what has ResFlow learns without violation on the feature dimension order is shown in Figure \ref{fig:case-study-2}. The left and middle parts represent the feature output of different hidden layers. The bottom four figure respectively represent the feature output of random net and MLP in different hidden layers of CTCVR tower. 

Residual links at different abstraction levels improve performance significantly by facilitating more efficient information transfer and selective knowledge utilization. With visualization in Figure \ref{fig:case study} and Figure \ref{fig:case-study-2}, dark areas of the residual visualization indicate that the model has learned to suppress the activation of the CTR task, while light-colored areas suggest strengthened activation of the CTR task. 
    
The color of our ResFlow change very smoothly in each hidden layer of CTCVR tower, which means that the residual link will enhance or inhibit the performance of CTCVR and increase the utilization of features; while the variance of the feature value in MLP is large, that is, the MLP cannot learn more complex patterns to fully utilize the features; in random net, due to random initialization to close to 0, the features cannot be effectively utilized.
    
\begin{figure*}
  \centering
  \includegraphics[width=\linewidth]{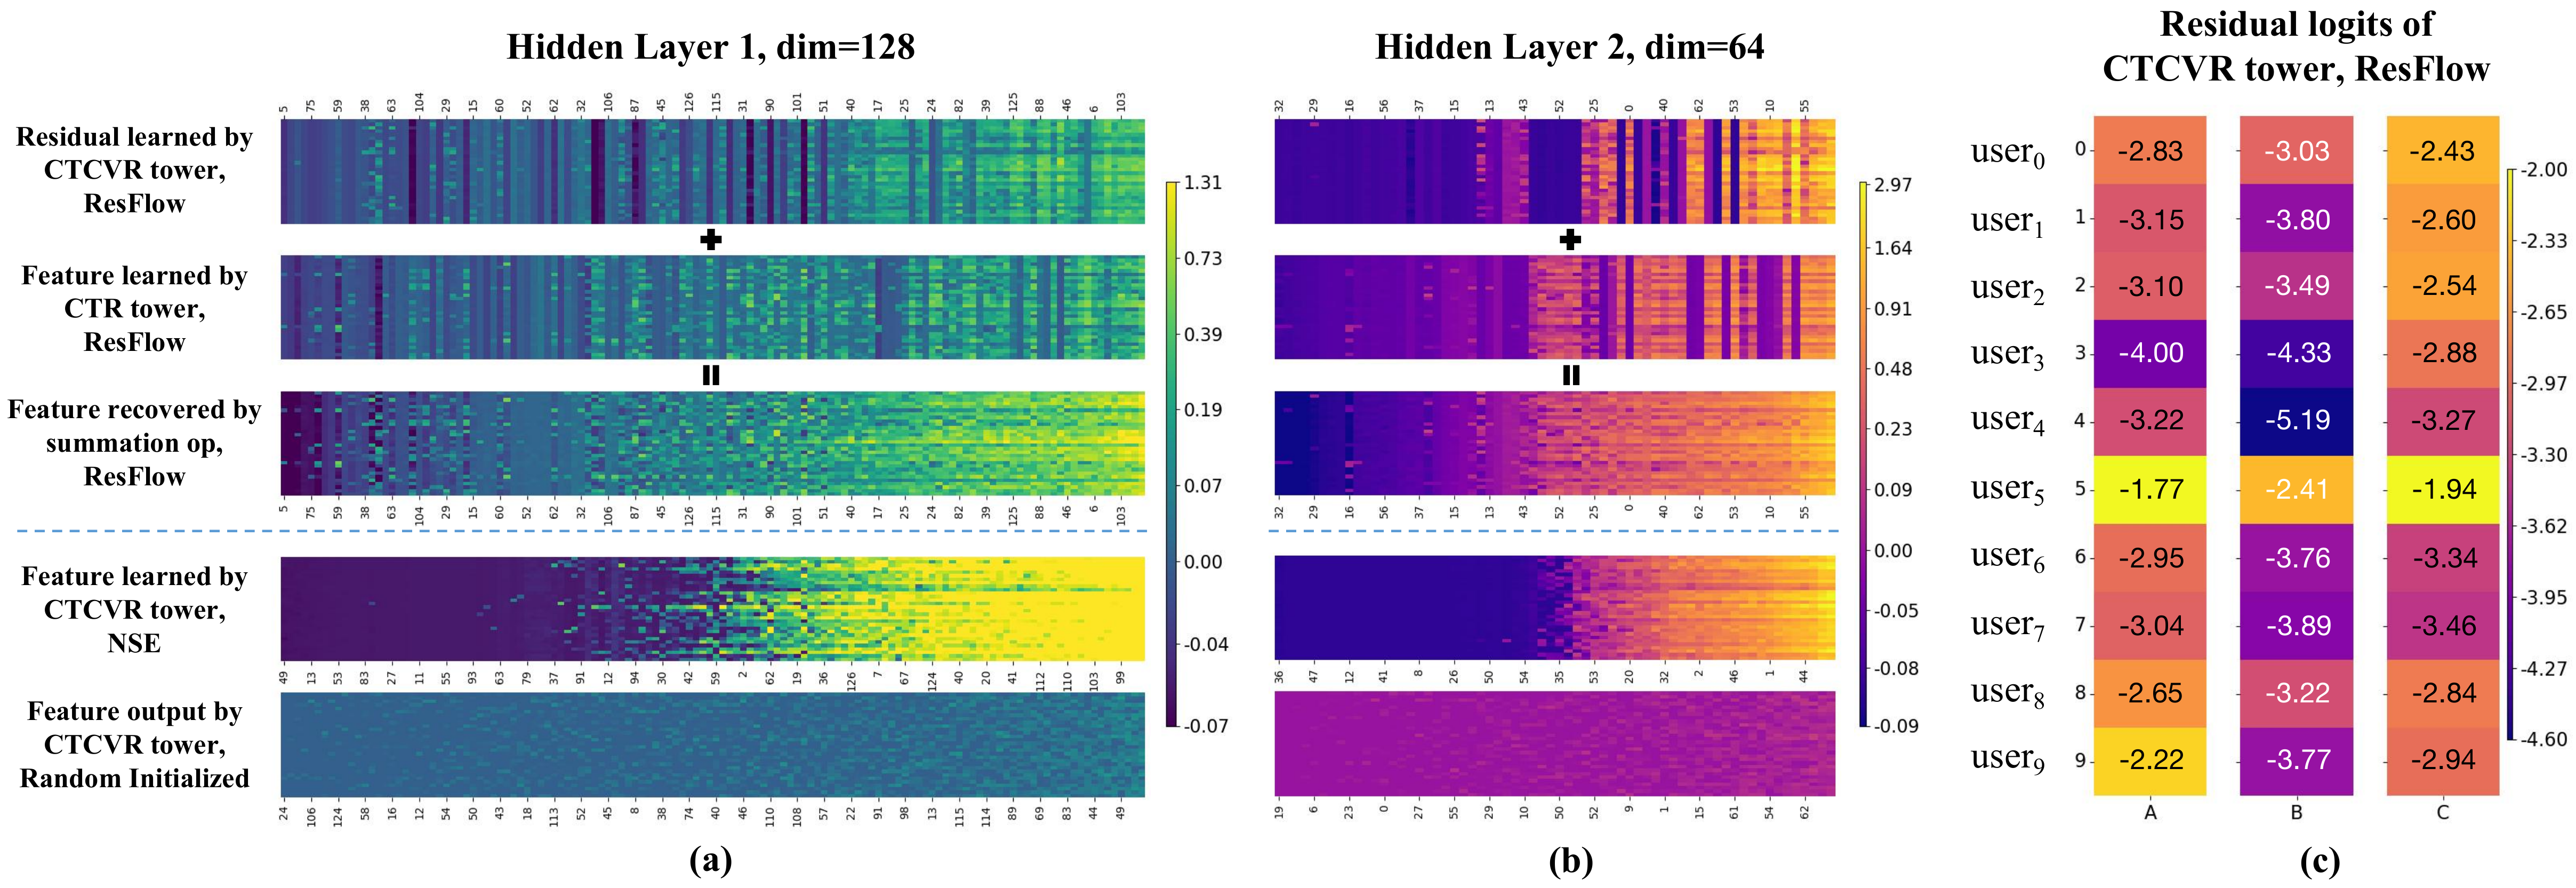}
  \caption{Case study on AliCCP dataset, a expanded version of Figure 3: We select 30 random samples (S00-S29) from 10 users to visualize the intermediate output of each layer. We visualize the feature learned by the CTR tower (the hidden layer output), the residual learned by the CTCVR tower (the hidden layer output) and the feature utilized by the CTCVR tower (the sum of the CTR output and the residual).  The dimension of the hidden layer outputs are in original order in contrast to Figure 3.}
  \label{fig:case-study-2}
\end{figure*}

\subsection{Online experiments}
\begin{figure*}
  \centering

  \includegraphics[width=\linewidth]{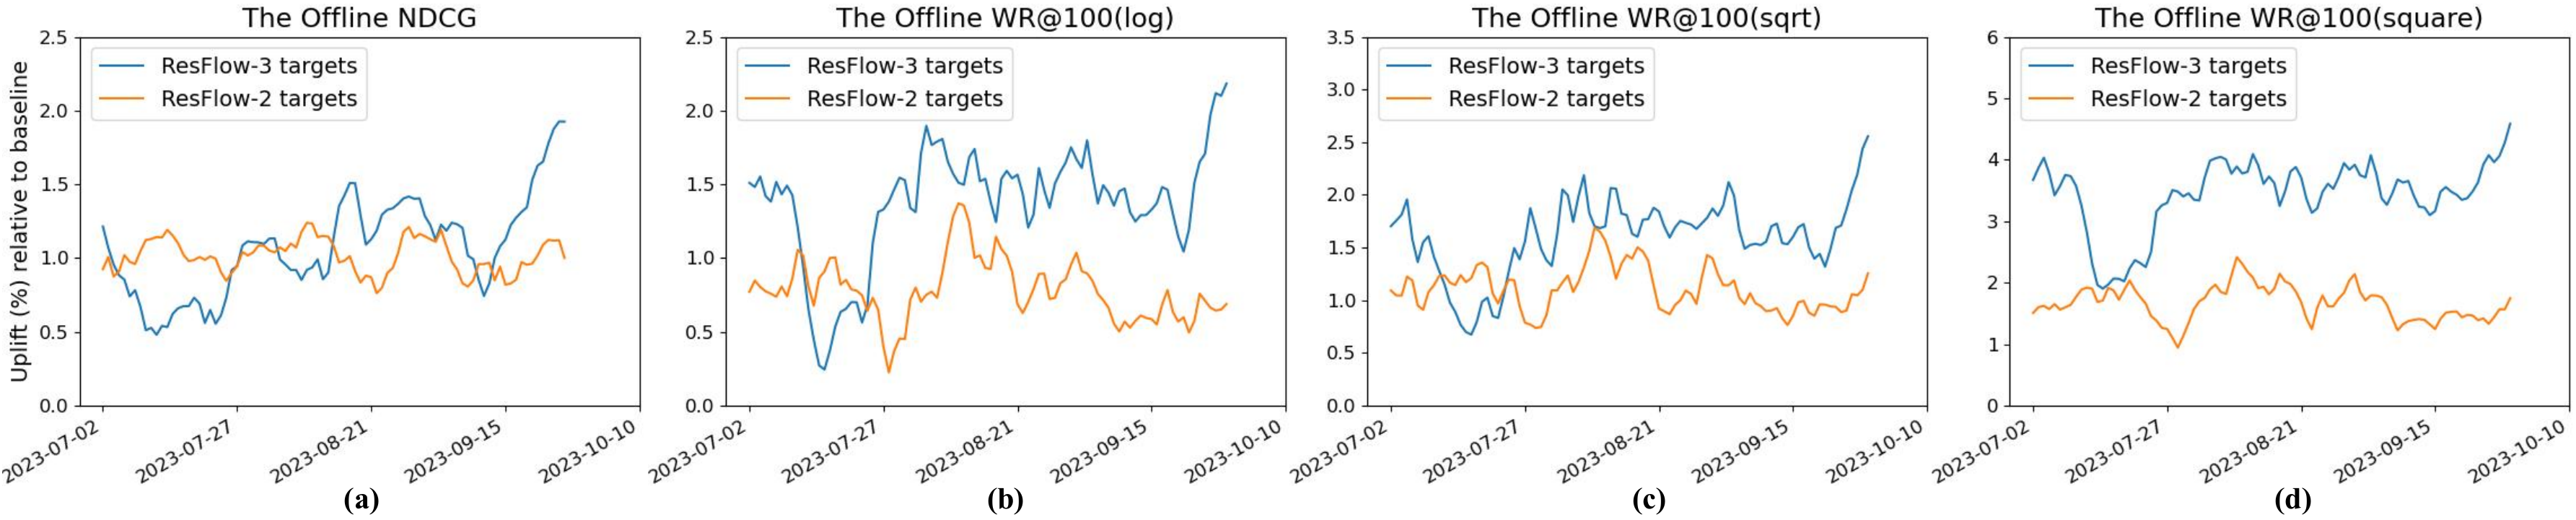}
  \caption{Daily Log of Online AB Test Uplift and Offline Main Metric. Non-smoothed version of Figure 4. From left to right: (a) the online OPU uplift, (b) the offline WRHI@100 uplift of fused scores, (c) offline CTCVR AUC uplift of fused scores. and (d) offline Recall@100 uplift of fused scores. }
  \label{fig: online-experiment2}
\end{figure*}

% \begin{table*}[h]
% \centering
% \caption{Online short term AB test for different score formula. The results are OPU uplift over baseline. The parameter configurations are the best ones found by grid search. Part of the subsequent searching combinations are shown in Figure 5.}
% \begin{tabular}{cccccccccc}
% \hline
% \hline
% Formula &Day1 & Day2 & Day3 & Day4 & Day5 & Day6 & Day7 &Day8 & Average\\
% \hline
% $CTR^{1.2}*CTCVR^{0.8}$ & 1.17 & 1.11 & -1.42 & 1.02 & 1.42 & -0.82 & 0.44 & 1.06 &\textbf{0.50}\\
% \hline
% $CTR+20*CTCVR$ & 0.77 & 1.19 & -0.46 & 1.01 & 1.45 &1.03 & 2.33 & 2.35 & \textbf{1.21}\\
% \hline
% \hline
% \end{tabular}
% \label{tab:online-exp-formula}
% \end{table*}

\textbf{Online experiments for different score formula.} We conduct an 8-day online A/B test to show the effect of different score formula indicated in Equation \ref{eq:score-formula1} and \ref{eq:score-formula2}. The test is done on 4\% traffic of Shopee main item search. The results are in Table \ref{tab:online-exp-formula}. Our new additive formula performs consistently better than the traditional multiplication formula, which supported the usage of the additive formula along with ResFlow framework. The results also indicate that the modeling of purchase behaviour should not be limited to the classic probability transfer framework. Instead, it can also be interpreted as the prediction of a ranking score with the help of CTR information via addition.

\subsection{Additional Offline Experiments}
We implement a few variants of ResFlow to evaluate their performance on Shopee dataset. The variants include $V_1$, $V_2$, $V_3$, and $V_4$. $V_1$ denotes the standard ResFlow used in previous experiments. $V_2$ stands for we optimise the CTR and CTCVR target separately. Specifically, we first freeze the parameters of CTCVR tower and optimise CTR tower to its best, then we freeze the parameters of CTR tower and optimise CTCVR tower to its best. $V_3$ represents we move ResFlow's residual link after the logits to the place before the logits. In other words, we first do the residual addition then do the dot-product. $V_4$ represents we add residual links both before and after the logit layer. The results are shown in Table \ref{tab:offline-exp-variants}

\begin{table*}[h]
\centering
\caption{Offline ResFlow two-target variant evaluation on Shopee dataset.}
\begin{tabular}{ccc}
\hline
\hline
Variants & CTR AUC & CTCVR AUC \\
\hline
$V_1$:ResFlow & $0.8656\pm0.0011$ & $0.9024\pm0.0010$\\
\hline
$V_2$:Separate Optimisation of Targets & $0.8155\pm0.0210$ & $0.9029\pm0.0009$\\
\hline
$V_3$:Move last residual link to after sigmoid & $0.8652\pm0.0013$ & $0.9021\pm0.0011$\\
\hline
$V_4$:Add residual link to before logits and after sigmoid & $0.8657\pm0.0011$ & $0.8812\pm0.0012$\\
\hline
\hline
\end{tabular}
\label{tab:offline-exp-variants}
\end{table*}

We can see that manipulating the position of the last residual link does not have a significant impact on the model performance. While add residual links to both before and after the logits hurt the CTCVR estimation a lot. Separate optimisation of different targets with ResFlow does not show improvement on the main target CTCVR, but leads to a significant drop in CTR estimation. This is maybe because the embedding is shared among tasks. In the second optimisation stage, freezing CTR tower parameters makes CTCVR optimisation dominates the learning of the embeddings. Therefore the solution space of the embedding parameters are dragged away from the Pareto Optima Space among tasks.

\begin{table*}[h]
\centering
\caption{Offline ResFlow two-target evaluation on different variants of Shopee dataset. We use the same test set to align the results. The test set is the full size data on day-10.}
\begin{tabular}{cc}
\hline
\hline
Manipulations  & CTCVR AUC \\
\hline
None & $0.9024\pm0.0010$\\
\hline
Down sampling the dataset to 10\% & $0.9002\pm0.0019$\\
\hline
Down sampling the dataset to 1\% & $0.8621\pm0.0111$\\
\hline
Down sampling the dataset to 0.1\% & $0.7713\pm0.03145$\\
\hline
Only use features whose importance ranks in top 50\% & $0.8732\pm0.0011$\\
\hline
Only use features whose importance ranks in top 25\% & $0.8411\pm0.0017$\\
\hline
Only use features whose importance ranks in top 10\% & $0.7938\pm0.0067$\\
\hline
\hline
\end{tabular}
\label{tab:offline-exp-dataset-manipulation}
\end{table*}

We also conduct experiments on Shopee dataset to show how manipulating the dataset will influence the performance of the model. We first evaluate the feature importance for all the features and do the feature reduction based on the importance. The results are shown in Table \ref{tab:offline-exp-dataset-manipulation}.

We can see that reduction on the quantity of features and samples will hurt the performance. The reason is that the feature are calculated or constructed based on full-size traffic logs upon historical data. Over down-sampling will obstacle the model from capturing rich feature patterns, especially for the sequential behaviour features.

However, in consideration of protecting confidential business information and the data storage, public datasets released by companies are usually employ reduction on features and samples both, such as Ali-CCP and AE datasets used in this paper. Models trained on such datasets are usually under-fit. This is also the reason why we find some methods work on public datasets while do not work in industry scale.

\subsection{On Online Score Formula}
In our case, the primary goal is OPU, thus the score formula used in online scenario is Equation \ref{eq:score-formula1} or \ref{eq:score-formula2}

However, for a e-commerce company pursuing profits, the price term is essential. The generally used score formula are Equation \ref{eq:score-formula3} and \ref{eq:score-formula4}.

\begin{equation}
\label{eq:score-formula3}
    Score = CTR^{\alpha} \cdot CVR^{\beta} \cdot Price^{\gamma}
\end{equation}

\begin{equation}
\label{eq:score-formula4}
    Score = (CTR^{\alpha} \cdot CVR^{\beta})^{\gamma} \cdot Price^{\epsilon}
\end{equation}


\section{ON THE CRITICISM OF ESCM THEORETICAL RESULTS}

We reckon that the proof presented by ESCM$^2$ regarding their claim of unbiasedness\cite{wang2022escm2} is not rigorous, which influences the foundation of their theoretical analysis and the design for ESCM-IPW and ESCM-DR model.  Their attempt to demonstrate that their Inverse Propensity
%Probability
Score (IPS) regularizer encourages unbiased Conversion Rate (CVR) estimation involves proving the equivalence of the IPS regularizer loss $\mathcal{R}_{IPS}$ to the ideal loss function $\mathcal{R}_{ideal}$ for modeling CVR over the entire impression space (as outlined in Theorem 2 in their paper). Upon a careful review of their proof, the following observations are noted.

To begin with, directly assume the CTR model yields the perfectly accurate estimation, i.e. $\hat{L}_{clk}(s_{jk})=o_{ij}$, is not meaningful, because then the both terms in denominator and numerator will cancel out inside the expectation, leaving no room for any proof.
% we will simply have
% \begin{align*}
% & \mathcal{R}_{IPS} \triangleq \mathbb{E}_{s_{jk} \in S^{imp}}\left\{\frac{o_{ij} \cdot \delta(L_{ord}(s_{jk}), \hat{L}_{ord}(s_{jk}))}{\hat{L}_{clk}(s_{jk})}\right\} \\
% & = \mathbb{E}_{s_{jk} \in S^{imp}}\left\{{ \delta(L_{ord}(s_{jk}), \hat{L}_{ord}(s_{jk}))}\right\} \triangleq \mathcal{R}_{ideal},\\
% \end{align*}
The sophisticated proof in ESCM$^2$ may mean for the case of uniformly convergence $\hat{L}_{clk}(s_{jk})\rightrightarrows o_{ij}$, where the manipulation/substitution of $\hat{L}_{clk}(s_{jk})$ only happens on the last step of the proof.

Moreover, suppose we strictly adhere to ESCM$^2$'s definition of IPS regularizer using the indicator function $o_{ij}\equiv L_{clk}(s_{jk}) = \mathbbm{1} [s_{jk} \in S^{clk}]$, we have the following when we revisit their proof of Theorem 2,\footnote{Note that the following discussions happen in the impression space $P(s_{jk})\triangleq P(s_{jk}|\mathbbm{1} [s_{jk} \in S^{imp}])$.}

\begin{align*}
& \mathcal{R}_{IPS} \triangleq \mathbb{E}_{s_{jk} \in S^{imp}}\left\{\frac{o_{ij} \cdot \delta(L_{ord}(s_{jk}), \hat{L}_{ord}(s_{jk}))}{\hat{L}_{clk}(s_{jk})}\right\} \\
& = \mathbb{E}_{s_{jk} \in S^{imp}}\left\{\frac{\mathbbm{1} [s_{jk} \in S^{clk}] \cdot \delta(L_{ord}(s_{jk}), \hat{L}_{ord}(s_{jk}))}{\hat{L}_{clk}(s_{jk})}\right\} \\
&\overset{\text{(1)}}{=} \int\int_{S^{clk}}\frac{ \delta(L_{ord}(s_{jk}), \hat{L}_{ord}(s_{jk}))}{\hat{L}_{clk}(s_{jk})}P(s_{jk}) dj dk \\
&\overset{\text{(2)}}{=} \int\int_{S^{clk}}\frac{ \delta(L_{ord}(s_{jk}), \hat{L}_{ord}(s_{jk}))}{1}P(s_{jk}) dj dk \\
& \overset{\text{(3)}}{\neq}\int\int_{S^{imp}}{ \delta(L_{ord}(s_{jk}), \hat{L}_{ord}(s_{jk}))}P(s_{jk}) dj dk  = \mathcal{R}_{ideal},\\
\end{align*}

The above step (1) holds from the property of indicator function, (2) holds from the assumption that the CTR is estimated accurately ($\hat{L}_{clk}(s_{jk})=\mathbbm{1} [s_{jk} \in S^{clk}]$), and (3) holds since generally we have $P(s_{jk})>0$ and $\delta(L_{ord}(s_{jk}), \hat{L}_{ord}(s_{jk}))>0$ on the domain ($S^{imp}\setminus S^{clk}$).
The above derivation shows that ESCM$^2$ has an inaccurate conclusion of $\mathcal{R}_{IPS} = \mathcal{R}_{ideal}$. In the above derivation, we have shown that their method may only yield an unbiased ideal loss function solely over the click sample space. 

% If we write the above conclusion in a more rigorous form, we can use the notion of uniformly convergence.

% \textbf{Revised Theorem 2.} Suppose $\hat{L}_{clk}(s_{jk})\in (0,1]$ is the prediction of click. Assume (1) $o_{ij}$ is the indicator function of click, (2) $\hat{L}_{clk}(s_{jk})$ is uniformly convergent to $o_{ij}$. Then we have
% \begin{align*}
% & 
% \mathcal{R}_{IPS} {\neq}\mathcal{R}_{ideal}.\\
% \end{align*}


\textbf{Reason of discrepancy}. If we known in advance that we are given the assumption that the CTR is estimated accurately ($\hat{L}_{clk}(s_{jk})=\mathbbm{1} [s_{jk} \in S^{clk}]$), the value of $\mathcal{R}_{IPS}$ is actually \textit{undefined}: on the domain of discrepancy ($S^{imp}\setminus S^{clk}$), both the denominator and numerator in the expectation are zero essentially because $\mathbbm{1} [s_{jk} \in S^{clk}]=0$.

To re-arrive at the Theorem 2 of ESCM$^2$, we have to avoid the undefined term by assuming there is an underlying probability $P({clk}|s_{jk})\in(0,1]$ for each observation of the click label. And now $o_{ij}$ should not be the indicator function, but the underlying probability $o_{ij}=P({clk}|s_{jk})$ instead\footnote{One equivalent deduction is to define $o_{ij}$ as the random variable / indicator function of the click event and then take the expectation over the user, item and label space, i.e. $\mathbb{E}_{s_{jk},o_{ij}}$, instead of just $\mathbb{E}_{s_{jk}}$. But it is clear that in the ESCM$^2$ the small $o$ notation stands for the observation instead of the random variable.}. Then, we should have the assumption of accurate prediction being $\hat{L}_{clk}(s_{jk})\rightrightarrows P({clk}|s_{jk})$.

In this regard, the replicated proof for Theorem 2 in ESCM$^2$ paper are presented below\cite{wang2022escm2}.

\begin{align*}
&\mathcal{R}_{IPS} \overset{\text{(1)}}{=} \mathbb{E}_{s_{jk} \in S^{imp}}\left\{\frac{o_{ij} \cdot \delta(L_{ord}(s_{jk}), \hat{L}_{ord}(s_{jk}))}{\hat{L}_{clk}(s_{jk})}\right\} \\
% &= \mathbb{E}_{s_{jk} \in S^{imp}}\left\{\frac{\mathbbm{1} [s_{jk} \in S^{clk}] \cdot \delta(L_{ord}(s_{jk}), \hat{L}_{ord}(s_{jk}))}{\hat{L}_{clk}(s_{jk})}\right\} \\
&= \int\int\frac{P({clk}|s_{jk}) \cdot \delta(L_{ord}(s_{jk}), \hat{L}_{ord}(s_{jk}))}{\hat{L}_{clk}(s_{jk})}P(s_{jk}) dj dk \\
&= \int\int\frac{\delta(L_{ord}(s_{jk}), \hat{L}_{ord}(s_{jk}))}{\hat{L}_{clk}(s_{jk})}P(s_{jk},clk) dj dk \\
&= \int\int\frac{\delta(L_{ord}(s_{jk}), \hat{L}_{ord}(s_{jk}))}{\hat{L}_{clk}(s_{jk})}P(s_{jk}|clk)P(clk) dj dk \\
&\overset{\text{(2)}}{=} \frac{|S^{clk}|}{|S^{imp}|}\int\int\frac{ \delta(L_{ord}(s_{jk}), \hat{L}_{ord}(s_{jk}))}{\hat{L}_{clk}(s_{jk})}P(s_{jk}|clk) dj dk \\
&\overset{\text{(3)}}{=} \frac{|S^{clk}|}{|S^{imp}|}\int\int\frac{ \delta(L_{ord}(s_{jk}), \hat{L}_{ord}(s_{jk}))}{P({clk}|s_{jk})}P(s_{jk}|clk) dj dk \\
&= \frac{|S^{clk}|}{|S^{imp}|}\int\int\frac{ \delta(L_{ord}(s_{jk}), \hat{L}_{ord}(s_{jk}))}{P({clk})}P(s_{jk}) dj dk \\
&\overset{\text{(4)}}{=} \int\int{ \delta(L_{ord}(s_{jk}), \hat{L}_{ord}(s_{jk}))}P(s_{jk}) dj dk 
\end{align*}
The above steps (1, 2, 3, 4) corresponds exactly to the 1st, 3rd, 4th, 5th lines of proof in the original ESCM$^2$ paper.

However, the assumptions brings some problems since in reality we cannot know the true underlying probability $P({clk}|s_{jk})$, and we can only obtain a coarse estimation of it given the one time observation of the label ${L}_{clk}(s_{jk})$. This largely undermines the persuasiveness of the IPS formulation: If $o_{ij}$ represents merely the label, the assumption of accurate estimation ($\hat{L}_{clk}(s_{jk})=\mathbbm{1} [s_{jk} \in S^{clk}]$) will be realistic since we only need to train a model to yield accurate prediction of the label. However, we have shown that for the theorem to hold, $o_{ij}$ should not represent merely the label, but should represent the underlying probability. In this sense, the assumption of accurate estimation ($\hat{L}_{clk}(s_{jk})=P({clk}|s_{jk})$) will be unrealistic since there is no way to accurately estimate $P({clk}|s_{jk})$ in the first place. As a result, the the
foundation of their theoretical analysis and the model design is undermined by such a unrealistic assumption.

% Our formula derivation is identical to theirs until equation (1) above; however, they omitted the condition $s_{jk} \in S^{clk}$ when expanding the expectation formula in (1). This omission led them to an incorrect conclusion that $\mathcal{R}_{IPS} = \mathcal{R}_{ideal}$. In our revised version, their method yields an unbiased CVR estimator solely over the click sample space.



\begin{comment}

\begin{table}[t]
    \centering
    \caption{Dataset statistics. Imp, Clk, and Cnv denote the number of impressions, clicks, and conversions, respectively. S0, S1, S2 denote the three different scenarios of AliCCP.}
    \begin{tabularx}{0.475\textwidth}{
        >{\centering\arraybackslash}m{2.5em}
        >{\centering\arraybackslash}m{2.2em}
        >{\centering\arraybackslash}m{2.2em}
        >{\centering\arraybackslash}m{2.2em}
        >{\centering\arraybackslash}m{2.2em}
        >{\centering\arraybackslash}m{1.8em}
        >{\centering\arraybackslash}m{1.8em}
        >{\centering\arraybackslash}m{3.5em}
    }
    \hline
    \hline
    Dataset & Split &  Imp & Clk & Cnv & CTR & CVR & CTCVR \\
    \hline
    \hline
     \multirow{2}{*}{AliCCP}& train & $42M$ & $1.6M$ & $9.0K$ & $3.9\%$ & $0.55\%$ & $0.021\%$ \\
     & test & $43M$ & $1.7M$ & $9.4K$ & $3.9\%$ & $0.56\%$ & $0.022\%$ \\
     \hline
     \multirow{2}{*}{S0} & train & $26M$ &$1.0M$ & $5.7K$ & $3.8\%$ & $0.57\%$ & $0.021\%$\\ 
    & test & $26M$ & $1.0M$ & $6.0K$ & $3.8\%$ & $0.60\%$ & $0.023\%$ \\
    \hline
     \multirow{2}{*}{S1} & train & $16M$ & $0.6M$ & $3.3K$ & $4.0\%$& $0.52\%$ & $0.021\%$ \\
     & test & $16M$ & $0.7M$ & $3.4K$ & $4.0\%$ & $0.52\%$ & $0.021\%$ \\
     \hline
    \multirow{2}{*}{S2} & train & $0.3M$ & $14K$  & $0$ & $4.6\%$  & $0\%$ & $0\%$\\
    & test & $0.3M$ & $14K$ & $0$ & $4.6\%$ & $0\%$ & $0\%$ \\
     \hline
    \multirow{2}{*}{S0\&S1} & train & $42M$ & $1.6M$ & $9.0K$ & $3.9\%$ & $0.55\%$ & $0.021\%$\\
    & test & $43M$ & $1.7M$ & $9.4K$ & $3.9\%$ & $0.56\%$ & $0.022\%$ \\
    \hline
    \hline
     \multirow{2}{*}{AE-ES} & train & $22M$ & $0.6M$ & $13K$ & $2.6\%$ & $2.25\%$ & $0.058\%$\\
     & test & $9.3M$ & $0.3M$ & $6.1K$ & $2.8\%$ & $2.30\%$ & $0.066\%$\\
     \hline
     \multirow{2}{*}{AE-FR} & train & $18M$ & $0.34M$ & $9.0K$ & $1.9\%$ & $2.63\% $& $0.049\%$ \\
     & test & $8.8M$ & $0.2M$ & $5.3K$ & $2.2\%$ & $2.71\%$ & $0.061\%$\\
     \hline
     \multirow{2}{*}{AE-NL} & train & $12.2M$ & $0.25M$ & $8.9K$ & $2.0\%$ & $3.63\%$ & $0.073\%$ \\
     & test & $5.6M$ & $0.14M$ & $4.9K$ & $2.4\%$ & $3.61\%$ & $0.088\%$\\
      \hline
    \multirow{2}{*}{AE-US} & train & $20.0M$ & $0.29M$ & $7.0K$ & $1.5\%$ & $2.41\%$ & $0.035\%$\\
     & test & $7.5M$ & $0.16M$ & $3.9K$ & $2.2\%$ & $2.41\%$ & $0.052\%$\\
      \hline
    \multirow{2}{*}{AE-RU} & train & $95M$ & $2.6M$ & $43K$ & $2.7\%$ & $1.68\%$ & $0.045\%$\\
     & test & $35M$ & $1.0M$ & $19K$ & $3.0\%$ & $1.79\%$ & $0.054\%$\\
    \hline
    \hline
    \multirow{2}{*}{Shopee} & train & $4.1B$ & $348M$ & $8.9M$ & $8.4\%$ & $2.57\%$ & $0.217
    \%$\\
    & test & $0.48B$ & $40M$ & $1.0M$ & $8.3\%$ & $2.65\%$ & $0.220\%$\\
    \hline
    \hline
    \end{tabularx}
    \label{tab:dataset}
\end{table}

The statistics of the datasets used in our offline evaluation are summarized in Table \ref{tab:dataset}. The datasets include:

\begin{itemize}[leftmargin=*]
    \item \textbf{AliCCP}\footnote{Dataset URL: [https://tianchi.aliyun.com/dataset/dataDetail?dataId=408]} \cite{ma2018entire} and \textbf{AE}\footnote{Dataset URL: [https://tianchi.aliyun.com/dataset/dataDetail?dataId=74690]} \cite{li2020improving} are provided by Alibaba Group. AliCCP, from Taobao's recommender system, is divided by scenarios into S0, S1, and S0\&S1. AE, from the AliExpress search system, is segmented by countries into AE-ES, AE-FR, AE-NL, and AE-US. The complete AliCCP dataset is also included in our evaluation.
    \item \textbf{Shopee}: Due to the scarcity of real-scale e-commerce datasets with comprehensive user feedback, we evaluated our model on the Shopee industrial dataset. This dataset was collected from 10 consecutive days of traffic logs on Shopee, processed as described in Section \ref{data curation}. The first 9 days serve as the training split, with the 10th day for testing. Shopee dataset encapsulates three types of user feedback: click, add-to-cart (ATC), and conversion. "Shopee-2" refers to using click and conversion labels, whereas "Shopee-3" includes ATC in the multi-task learning process.
\end{itemize}


% Two public e-commerce datasets (AliCPP and AE), as well as a private dataset from Shopee, are considered in our experiments. The statistics of these datasets are provided in Table \ref{tab:dataset}. 

% \textbf{AliCCP} (Alibaba Click and Conversion Prediction\footnote{Dataset URL: https://tianchi.aliyun.com/dataset/dataDetail?dataId=408}) \cite{ma2018entire}. This dataset is derived from the real-world traffic logs of the recommender system in Taobao. It encompasses a wide range of features, including user features, item features, cross features, and context features, while the labels include clicks and conversions. Following the setting of AITM \cite{xi2021modeling}, we use a subset of 19 selected features in our experiments. Notably, this dataset contains three different scenarios, which we denote as S0, S1, and S2. As shown in Table \ref{tab:dataset}, they have different sizes, and particularly S2 does not have conversion labels. To address the complexity introduced by such multi-scenarios, we further consider sub-scenarios in our experiments besides the entire dataset, including S0, S1, and S0\&S1, where S0\&S1 means using S0 and S1. When leveraging the entire AliCCP dataset, S2 is only used in the CTR estimation task. 

% \textbf{AE} (Ali-Express\footnote{Dataset URL: https://tianchi.aliyun.com/dataset/dataDetail?dataId=74690}) \cite{li2020improving}. This dataset is obtained from the real-world traffic logs of the search system in AliExpress, collected from five countries, which are denoted as AE-RU, AE-ES, AE-FR, AE-NL, and AE-US, respectively. It includes user features, item features, and labels denoting clicks and conversions. We use all 62 features available in the dataset and bucketize each numeric feature into 100 buckets. 

% \textbf{Shopee.} Due to the scarcity of e-commerce datasets that provide diverse feedback beyond clicks and conversions, and the lack of a large enough offline dataset, we created a dataset based on the daily traffic logs and rank server logs from the primary search scenario in one of Shopee's main business regions. It is generated with negative sampling based on the original 10-day logs, and by design includes 10\% click samples, 40\% impression-not-click samples, 40\% unimpression samples, and 10\% artificial random samples. As for the train-test split, we use samples of the first 9 days as the training set and the tenth day as the testing set. It encompasses user, query, and item features, amounting to more than 200 features, and the labels include three types: click, add-to-cart, and conversion. We use Shoppe-2 to indicate results on Shoppe but using only the click and conversion labels, i.e., there are two estimation tasks: CTR and CTCVR, as other datasets, and Shoppe-3 to indicate results using all its three labels (click, add-to-cart, and conversion) with three estimation tasks: CTR, ATCR, and CTCVR. 

For further details on the datasets, please refer to the Appendix.

% The composition of samples is a fundamental aspect in optimizing the efficiency of the pre-rank module\cite{zhang2023rethinking}. 

% To more effectively focus on the method's performance, the Shopee dataset has been meticulously optimized and organized to unlock the full potential of all methods.

% specifically designed for the pre-rank stage, 

\subsubsection{Baseline Methods}

The baseline methods considered in our experiments include: ESMM \cite{ma2018entire}; AITM \cite{xi2021modeling}; ESCM$^2$-IPW \cite{wang2022escm2}; ESCM$^2$-DR \cite{wang2022escm2}; DCMT \cite{zhu2023dcmt}. Besides, we include MLP that directly learns each task with a multi-layer perceptron. We exclude multi-task methods such as MMOE \cite{ma2018modeling} and PLE \cite{tang2020progressive} due to their empirically inferior performance as reported in the aforementioned baseline papers \cite{xi2021modeling,wang2022escm2,zhu2023dcmt}. 

\subsubsection{Evaluation Metrics}

% Since CVR estimation is excluded from the ResFlow framework, we exclusively report the CTCVR estimation performance of all methods on E-commerce datasets.  

In line with conventions \cite{ma2018entire,wang2022escm2,zhu2023dcmt}, the evaluation metric used in the experiments is the area under the ROC curve (AUC). All experiments are conducted five times with different random seeds, and the average value along with the standard deviation is provided. 

\subsubsection{Implementation Details}

To ensure a fair comparison, we use the same backbone network architecture and the same basic configurations for all methods in our experiments. Specifically: For the AliCCP dataset, we adopt a two-layer MLP of hidden size (128,64) as the backbone for all methods, with an embedding size of 32, a batch size of 2048, and a learning rate of 4e-4. For the AE dataset, we adopt a three-layer MLP of hidden size (256,128,16) as the backbone for all methods, with an embedding size of 32, a batch size of 1024, and a learning rate of 1e-3. For the Shopee dataset, we adopt a three-layer MLP of hidden size (256,128,16) as the backbone for all methods, with an embedding size of 16, a batch size of 512, and a learning rate of 5e-4. More detailed configurations are provided in the Appendix. 

% while fine-tuning key parameters on different datasets for optimal performance
% We provide results from both our implementation and the best-known results in previous papers as a reference. 
% 
% Across all methods and datasets, we maintain an embedding size of 32, utilize PReLU as the activation function, and limit the maximum training epochs to 10. 

\end{comment}



table \ref{tab:calibration-loss} \ref{tab:regression-para-search}
\begin{table}[h]
\centering
\caption{Add calibration to probability to ensure monotonicity.}
\begin{tabular}{cccc}
\hline
\hline
Method & Dataset & cali loss weight & MSE \\
\hline
AITM-like & kuaishou & 1:1 & 1657.84 \\
AITM-like & kuaishou & 1:2 & 1662.45 \\
AITM-like & kuaishou & 1:0.5 & 1658.95 \\
AITM-like & kuaishou & 1:0.1 & 1658.45 \\
\hline
-max(logit,0) & kuaishou & 1:1 & 2234.38 \\
-max(logit,0) & kuaishou & 1:2 & 20258.95\\ 
-max(logit,0) & kuaishou & 1:0.5 &1660.26 \\ 
-max(logit,0) & kuaishou & 1:0.1 &1656.72 \\
\hline
ESMM + feature residual  & kuaishou & - & 1673.55 \\
\hline
residual min(logit,0)  & kuaishou & - & 1655.8307 \\
\hline
residual min(logit,0)  & Shopee-3 & - & 0.9102 \\
AITM-like & Shopee-3 & 1:0.1 & 0.9093 \\
-max(logit,0) & Shopee-3 & 1:0.1 & 0.9087 \\
ESMM + feature residual & Shopee-3 & - & 0.90852 \\
\hline
\hline
Method & Dataset & cali loss weight & AUC \\
\hline
AITM-like & AE-RU & 1:1 & 0.9128 \\
AITM-like & AE-RU & 1:2 & 0.9124 \\
AITM-like & AE-RU & 1:0.5 & 0.9133 \\
AITM-like & AE-RU & 1:0.1 & 0.9131 \\
\hline
-max(logit,0) & AE-RU & 1:1 & 0.8817 \\
-max(logit,0) & AE-RU & 1:2 & 0.7176\\ 
-max(logit,0) & AE-RU & 1:0.5 & 0.8898 \\ 
-max(logit,0) & AE-RU & 1:0.1 & 0.9097 \\
\hline
ESMM + feature residual  & AE-RU & - & 0.9083 \\
\hline
residual min(logit,0)  & AE-RU & - & 0.9134516 \\
\hline
\hline
\end{tabular}
\label{tab:calibration-loss}
\end{table}

\begin{table}[h]
\centering
\caption{Regression best parameter search}
\begin{tabular}{ccc}
\hline
\hline
param & Dataset & score  \\
\hline
[256,256,1] & ML-1M & 0.9172 \\
\hline
[96, 48, 1] & ML-1M & 0.9087 \\
\hline
[192,128,1] & ML-1M & 0.9072 \\
\hline
[192,128,1] & ML-1M & 0.9079 \\
\hline
[1152,64,1] & ML-1M & 0.9081 \\
\hline
[192,96,1] & kuaishou & 1732.851 \\
\hline
[64,64,1] & kuaishou &  1719.3489 \\
\hline
[128,128,1] & kuaishou &  1729.2385 \\
\hline
[256,128,1] & kuaishou & 1743.790 \\
\hline
\hline
\end{tabular}
\label{tab:regression-para-search}
\end{table}
